# Supplementary material for: TIAGo RL: Simulated Reinforcement Learning Environments with Tactile Data for Mobile Robots
Source: arXiv:2311.07260 source file (2023-11-13)
Supplement: Supplementary file 1 [file 99_appendix_ack.tex]

% \section*{APPENDIX}
% Appendixes should appear before the acknowledgment.
% \section*{ACKNOWLEDGMENT}
